# Supplementary material for: Zeta and L-functions of finite quotients of apartments and buildings
Source: arXiv:1505.00902 ancillary file (2017-05-04)
Supplement: Supplementary file 1 [file Table_2_Computation.pdf]

# ZETA AND L-FUNCTIONS OF FINITE QUOTIENTS OF APARTMENTS AND BUILDINGS (COMPUTATION OF TABLE 2)

MING-HSUAN KANG, WEN-CHING WINNIE LI AND CHIAN-JEN WANG

In this note we compute the eigenvalues of the vertex adjacency operators  $A_1, A_2, A'_2, A''_2$ , the edge adjacency operators  $L_{P_1}, L_{P_2}$ , and the chamber adjacency operator  $L'_I$  on each type of representations classified in Table 1 of [2] to establish Table 2 of [2]. All the notations are as in [2]. Set

$$R(u) = \frac{\det(I + L'_I u) \det(I - A'_2 u + (qA_1^2 - 2q^2 A_2'')u^2 - q^4 A'_2 u^3 + q^8 I u^4)}{\det(I - L_{P_1}^2 u^2) \det(I - L_{P_2} u)}.$$

We record all the eigenvalues information as well as the contribution to  $R(u)$  from each type of representations in the table given in §3. The computation for the eigenvalues of  $A_1, A_2, L_{P_1}, L_{P_2}$  has actually been done in [1] so we just borrow the results. A different chamber adjacency operator  $L_I$  is considered in [1], but the method of computation works exactly the same here for  $L'_I$ . So we follow closely the approach and illustration of [1, §5], only make necessary changes to record new data.

## 1. PRINCIPAL SERIES REPRESENTATIONS

Since each irreducible Iwahori-spherical representation of  $G = \mathrm{GSp}_4(\mathbb{F})$  can be embedded into an unramified principal series representation of  $G$ , we begin with a principal series representation  $\rho_0 \simeq \chi_1 \times \chi_2 \rtimes \sigma$  induced from unramified characters  $\chi_1, \chi_2, \sigma$  of  $F^\times$  with  $\chi_1 \chi_2 \sigma^2 = \mathbf{1}_{F^\times}$ . It can be realized in the space  $V$  consisting of functions  $f : G \rightarrow \mathbb{C}$  satisfying the transformation property

$$f(hg) = |a^2 b c^{-\frac{3}{2}}| \chi_1(a) \chi_2(b) \sigma(c) f(g), \quad \text{for all } h = \begin{pmatrix} a & * & * & * \\ 0 & b & * & * \\ 0 & 0 & cb^{-1} & * \\ 0 & 0 & 0 & ca^{-1} \end{pmatrix} \in B,$$

where  $B$  is the Borel subgroup of  $G$ . Let  $W$  be the Weyl group of  $G$  generated by  $s_1 = \begin{pmatrix} 1 & & & \\ & 1 & & \\ & & 1 & \\ & & & 1 \end{pmatrix}$ ,  $s_2 = \begin{pmatrix} 1 & & & \\ & 1 & & \\ & & 1 & \\ & & & 1 \end{pmatrix}$ . Let  $f_\alpha(x)$  be the function in  $V$  supported on the coset  $B\alpha I$  with  $f_\alpha(\alpha I) = 1$ . It follows from the decomposition  $G = \bigsqcup_{w \in W} BwI$  that the space of Iwahori-invariant vectors  $V^I$  has dimension eight, with a basis consisting of  $f_1 := f_{id}$ ,  $f_2 := f_{s_1}$ ,  $f_3 := f_{s_2}$ ,  $f_4 := f_{s_1 s_2}$ ,  $f_5 := f_{s_2 s_1}$ ,  $f_6 := f_{s_1 s_2 s_1}$ ,  $f_7 := f_{s_2 s_1 s_2}$ ,  $f_8 := f_{s_1 s_2 s_1 s_2}$ .

Let  $e_i$  be the characteristic function of  $Is_i I$  for  $i = 0, 1, 2$  and let  $\eta$  be the characteristic function of  $I\tau I = \tau I$ , where  $s_0 = \begin{pmatrix} 1 & & & \\ & 1 & & \\ & & 1 & \\ & & & 1 \end{pmatrix}$  and  $\tau = \begin{pmatrix} 1 & & & \\ & 1 & & \\ \varpi & & 1 & \\ & \varpi & & 1 \end{pmatrix}$ . Then the Iwahori-Hecke algebra of  $G$  is generated by  $e_0, e_1, e_2$  and  $\eta$ . Note that

$$Is_1 I = \bigsqcup_{a \in \mathcal{O}/\mathcal{P}} \begin{pmatrix} 1 & a & 0 & 0 \\ 0 & 1 & 0 & 0 \\ 0 & 0 & 1 & -a \\ 0 & 0 & 0 & 1 \end{pmatrix} s_1 I, \quad Is_2 I = \bigsqcup_{a \in \mathcal{O}/\mathcal{P}} \begin{pmatrix} 1 & 0 & 0 & 0 \\ 0 & 1 & a & 0 \\ 0 & 0 & 1 & 0 \\ 0 & 0 & 0 & 1 \end{pmatrix} s_2 I,$$

so with respect to the ordered basis  $\{f_1, f_2, f_3, f_5, f_6, f_4, f_8, f_7\}$ , the Iwahori-Hecke operators  $e_1, e_2, \eta$  have matrix representations

$$M_{e_1} = \begin{pmatrix} 0 & q & & & & & & \\ 1 & q^{-1} & & & & & & \\ & & 0 & q & & & & \\ & & 1 & q^{-1} & & & & \\ & & & & q^{-1} & 1 & & \\ & & & & q & 0 & & \\ & & & & & & q^{-1} & 1 \\ & & & & & & q & 0 \end{pmatrix}, \quad M_{e_2} = \begin{pmatrix} 0 & 0 & q & 0 & 0 & 0 & 0 & 0 \\ 0 & 0 & 0 & 0 & 0 & q & 0 & 0 \\ 1 & 0 & q^{-1} & 0 & 0 & 0 & 0 & 0 \\ 0 & 0 & 0 & 0 & 0 & 0 & 0 & q \\ 0 & 0 & 0 & 0 & 0 & 0 & q & 0 \\ 0 & 1 & 0 & 0 & 0 & q^{-1} & 0 & 0 \\ 0 & 0 & 0 & 0 & 1 & 0 & q^{-1} & 0 \\ 0 & 0 & 0 & 1 & 0 & 0 & 0 & q^{-1} \end{pmatrix},$$

and

$$M_\eta = \begin{pmatrix} & & & & & & & \gamma q^{3/2} \\ & & & & & & \gamma q^{3/2} & \\ & & & & & \beta \gamma q^{1/2} & & \\ & & & & \alpha \gamma q^{-1/2} & & & \\ & & & \alpha \gamma q^{-1/2} & & & & \\ & & \alpha \beta \gamma q^{-3/2} & & & & & \\ \alpha \beta \gamma q^{-3/2} & & & & & & & \end{pmatrix},$$

where  $\alpha = \chi_1(\varpi), \beta = \chi_2(\varpi), \gamma = \sigma(\varpi)$ . The matrix representation for  $e_0$  is given by  $M_{e_0} = M_\eta M_{e_2} M_\eta^{-1}$ .

1.0.1. *Eigenvalues of  $L'_I$ .* The Iwahori-Hecke operator  $L'_I$  is represented by the characteristic function of  $It'I$ , where  $t' = s_0 s_1 s_2$ . Since the decomposition of  $t'$  as the product of  $s_0, s_1, s_2$  is reduced, the matrix representations of  $L'_I$  with respect to the basis  $\{f_1, f_2, f_3, f_5, f_6, f_4, f_8, f_7\}$  is given by  $M_{s_0} M_{s_1} M_{s_2}$ . Then we have the following explicit description of  $L'_I$ .

(1.1)

$$\begin{aligned} L'_I f_1 &= q \chi_2^{-1}(\varpi) f_2, & L'_I f_2 &= q^2 \chi_1^{-1}(\varpi) f_1, \\ L'_I f_3 &= (q^2 - q + (q^2 - q) \chi_2^{-1}(\varpi)) f_2 + q \chi_2(\varpi) f_5, \\ L'_I f_4 &= (q^3 - q^2 + (q^3 - q^2) \chi_1^{-1}(\varpi)) f_1 + q(q-1)^2 f_2 + (q^2 - q) \chi_2(\varpi) f_5 + q \chi_1(\varpi) f_6, \\ L'_I f_5 &= q^2 \chi_1^{-1}(\varpi) f_3, \\ L'_I f_6 &= (q^3 - q^2) \chi_1^{-1}(\varpi) f_3 + q^2 \chi_2^{-1}(\varpi) f_4, \\ L'_I f_7 &= (q^3 - q^2) \chi_2^{-1}(\varpi) f_2 + (q^3 - q^2 + (q^3 - q^2) \chi_1^{-1}(\varpi)) f_3 + q \chi_1(\varpi) f_8, \\ L'_I f_8 &= (q^4 - q^3) \chi_1^{-1}(\varpi) f_1 + q^2(q-1)^2 \chi_1^{-1}(\varpi) f_3 + (q^3 - q^2 + (q^3 - q^2) \chi_2^{-1}(\varpi)) f_4 + q^2 \chi_2(\varpi) f_7. \end{aligned}$$

One can verify that the eigenvalues of  $L'_I$  on  $V^I$  are  $\pm q^{3/2} \sigma(\varpi), \pm q^{3/2} \chi_1 \sigma(\varpi), \pm q^{3/2} \chi_2 \sigma(\varpi)$ , and  $\pm q^{3/2} \chi_1 \chi_2 \sigma(\varpi)$ .

1.0.2. *Eigenvalues of  $A_1, A_2, A'_2, A''_2$ .* The subspace  $V^K$  is one-dimensional, generated by  $\sum_{i=1}^8 f_i$ . It has been computed in [1, §5.1.3] that the Hecke operators  $A_1, A_2$  act on  $V^K$  via the scalar multiplications by  $\lambda_1$  and  $\lambda_2$  respectively, where

$$(1.2) \quad \begin{aligned} \lambda_1 &= q^{\frac{3}{2}} (\chi_1 \chi_2(\varpi) + \chi_1(\varpi) + \chi_2(\varpi) + 1) \sigma(\varpi), \\ \lambda_2 &= q^2 (\chi_1^2 \chi_2(\varpi) + \chi_1 \chi_2^2(\varpi) + \chi_1(\varpi) + \chi_2(\varpi) + 2 \chi_1 \chi_2(\varpi)) \sigma^2(\varpi). \end{aligned}$$

Then the Hecke operators  $A'_2 = A_2 - 2q^2 I$  and  $A''_2 = A_2 - q^2 I$  act on  $V^K$  by scalars  $\lambda'_2 = \lambda_2 - 2q^2$  and  $\lambda''_2 = \lambda_2 - q^2$  respectively.

## 2. EIGENVALUES COMPUTATION

From now on, let  $(\rho, V_\rho)$  be a unitary irreducible Iwahori-spherical representation in  $L^2(\Gamma \backslash G/Z)$ , which is one of the fifteen sub-types listed in Table 1 of [2]. Among the fifteen sub-types, unramified representations are of type I, IIb, IIIb, IVd, Vd, or VIId. If  $\rho$  belongs to type I, it is isomorphic to  $\chi_1 \times \chi_2 \rtimes \sigma$  with  $\chi_1 \chi_2 \sigma^2 = \mathbf{1}_{F^\times}$ . Applying results from §1.0.2, one checks directly that the reciprocals of zeros of  $\det(I - A'_2 u + (qA_1^2 - 2q^2 A_2'')u^2 - q^4 A_2' u^3 + q^8 I u^4)$  on  $V_\rho$  are  $q^2 \chi_1 \sigma^2(\varpi), q^2 \chi_2 \sigma^2(\varpi), q^2 \chi_1 \chi_2^2 \sigma^2(\varpi)$ , and  $q^2 \chi_1^2 \chi_2 \sigma^2(\varpi)$ . For types IIb, IIIb, IVd, Vd, VIId representations, they are subrepresentations of principal series representations  $\nu^{-1/2} \chi \times \nu^{1/2} \chi \rtimes \sigma, \chi \times \nu^{-1} \rtimes \nu^{1/2} \sigma, \nu^{-2} \times \nu^{-1} \rtimes \nu^{3/2} \sigma, \xi \nu^{-1} \times \xi \rtimes \nu^{1/2} \xi \sigma, \nu^{-1} \times \mathbf{1}_{F^\times} \rtimes \nu^{1/2} \sigma$  respectively. Similar calculation shows that the reciprocals of zeros of  $\det(I - A'_2 u + (qA_1^2 - 2q^2 A_2'')u^2 - q^4 A_2' u^3 + q^8 I u^4)$  on  $V_\rho$  are as shown in the table given in §3. In what follows, we shall compute the eigenvalues of  $L'_I$  on  $V_\rho^I$  case by case.

**2.1. Type I representations.** Suppose  $\rho$  has type I, then it has the form  $\chi_1 \times \chi_2 \rtimes \sigma$  with  $\chi_1 \chi_2 \sigma^2 = \mathbf{1}_{F^\times}$ . It follows from §1.0.1 that the eigenvalues of  $L'_I$  on  $V_\rho^I$  are  $\pm q^{3/2} \sigma(\varpi), \pm q^{3/2} \chi_1 \sigma(\varpi), \pm q^{3/2} \chi_2 \sigma(\varpi)$ , and  $\pm q^{3/2} \chi_1 \chi_2 \sigma(\varpi)$ .

**2.2. Type II representations.** Suppose  $\rho$  has type II, then it is a constituent of  $\nu^{-\frac{1}{2}} \chi \times \nu^{\frac{1}{2}} \chi \rtimes \sigma$  with  $\chi^2 \sigma^2 = \mathbf{1}_{F^\times}$ . There are two constituents in the representation  $\nu^{-\frac{1}{2}} \chi \times \nu^{\frac{1}{2}} \chi \rtimes \sigma$ .

**2.2.1. Type IIb.** Suppose  $\rho \simeq \chi \mathbf{1}_{\text{GL}_2} \rtimes \sigma$ , which is the unique subrepresentation of  $\nu^{-\frac{1}{2}} \chi \times \nu^{\frac{1}{2}} \chi \rtimes \sigma$ . It can be realized in the parabolically induced space  $V_\rho$  consisting of functions  $f : G \rightarrow \mathbb{C}$  satisfying

$$f(hg) = |\det(A)^{\frac{3}{2}} c^{-\frac{3}{2}}| \chi(\det(A)) \sigma(c) f(g) \quad \text{for all } h = \begin{pmatrix} A & * \\ 0 & cA' \end{pmatrix} \in P,$$

where  $A' = \begin{pmatrix} 0 & 1 \\ 1 & 0 \end{pmatrix}^t A^{-1} \begin{pmatrix} 0 & 1 \\ 1 & 0 \end{pmatrix}$  and  $P$  is the Siegel parabolic subgroup of  $G$ . Let  $f_\alpha$  denote the function in  $V_\rho^I$  supported on the coset  $P\alpha I$ , taking value 1 at  $\alpha$ .

It follows from the decomposition  $G = \bigsqcup_{w \in W_1 \backslash W} PwI$  that the space  $V_\rho^I$  has dimension four, generated by  $f_1 := f_{id}, f_2 := f_{s_2}, f_3 := f_{s_2 s_1}, f_4 := f_{s_2 s_1 s_2}$ . Similar computation as in §1.0.1 gives the explicit actions of  $L'_I$  on the given basis:

$$\begin{aligned} L'_I(f_1) &= q^{3/2} \chi^{-1}(\varpi) f_1, & L'_I(f_2) &= (q^3 - q^2 + (q^{5/2} - q^{3/2}) \chi^{-1}(\varpi)) f_1 + q^{3/2} \chi(\varpi) f_3, \\ L'_I(f_3) &= q^{5/2} \chi^{-1}(\varpi) f_2, \\ L'_I(f_4) &= (q^{7/2} - q^{5/2}) \chi^{-1}(\varpi) f_1 + (q^3 - q^2 + (q^{7/2} - q^{5/2}) \chi^{-1}(\varpi)) f_2 + q^{3/2} \chi(\varpi) f_4. \end{aligned}$$

Therefore  $L'_I$  on  $V_\rho$  has eigenvalues  $\pm q^2, q^{3/2} \chi^{-1}(\varpi), q^{3/2} \chi(\varpi)$ .

**2.2.2. Type IIa.** Suppose now  $\rho \simeq \chi \text{St}_{\text{GL}_2} \rtimes \sigma$ . Since  $\chi \text{St}_{\text{GL}_2} \rtimes \sigma$  and  $\chi \mathbf{1}_{\text{GL}_2} \rtimes \sigma$  are the two constituents of  $\nu^{-\frac{1}{2}} \chi \times \nu^{\frac{1}{2}} \chi \rtimes \sigma$ , the eigenvalues of  $L_I$  on  $V_\rho^I$  can be obtained by first finding the eigenvalues of  $L'_I$  on the full induced space  $\nu^{-\frac{1}{2}} \chi \times \nu^{\frac{1}{2}} \chi \rtimes \sigma$ , then excluding those eigenvalues coming from the type IIb representation  $\chi \mathbf{1}_{\text{GL}_2} \rtimes \sigma$  studied in §2.2.1. The first step can be done using the result of §1.0.1 with  $\chi_1 = \nu^{-\frac{1}{2}} \chi$  and  $\chi_2 = \nu^{\frac{1}{2}} \chi$ . We deduce that the eigenvalues of  $L'_I$  on  $V_\rho^I$  are  $\pm q, -q^{3/2} \chi(\varpi), -q^{3/2} \chi^{-1}(\varpi)$ .

**2.3. Type III representations.** Suppose  $\rho$  has type III so that it is a constituent of  $\chi \times \nu^{-1} \rtimes \nu^{\frac{1}{2}} \sigma$  with  $\chi \sigma^2 = \mathbf{1}_{F^\times}$ . There are two constituents in the representation  $\chi \times \nu^{-1} \rtimes \nu^{\frac{1}{2}} \sigma$ .

2.3.1. *Type IIIb.* Consider first  $\rho \simeq \chi \rtimes \sigma \mathbf{1}_{\mathrm{GSp}_2}$ . It is the unique subrepresentation of  $\chi \times \nu^{-1} \rtimes \nu^{\frac{1}{2}}\sigma$ , and can be realized in the space  $V_\rho$  consisting of functions  $f : G \rightarrow \mathbb{C}$  satisfying

$$f(hg) = |t^2(ad - bc)^{-1}| \chi(t) \sigma(ad - bc) f(g) \quad \text{for all } h = \begin{pmatrix} t & * & * & * \\ 0 & a & b & * \\ 0 & c & d & * \\ 0 & 0 & 0 & \Delta t^{-1} \end{pmatrix} \in Q,$$

where  $\Delta = ad - bc$ , and  $Q$  is the Klingen parabolic subgroup of  $G$ . Let  $f_\alpha$  be defined as in §2.2.1 type IIb case, with the Siegel parabolic  $P$  there replaced by the Klingen parabolic  $Q$ .

The space of Iwahori invariant vectors  $V_\rho^I$  has dimension four since  $G = \bigsqcup_{w \in W_2 \backslash W} QwI$ , where  $W_2 \backslash W = \{id, s_1, s_1s_2, s_1s_2s_1\}$ . It has a basis given by  $f_1 := f_{id}, f_2 := f_{s_1}, f_3 := f_{s_1s_2}$  and  $f_4 := f_{s_1s_2s_1}$ . With this basis, the action of  $L'_I$  can be described as follows.

$$\begin{aligned} L'_I(f_1) &= q^2 f_2, \\ L'_I(f_2) &= q^2 \chi^{-1}(\varpi) f_1, \\ L'_I(f_3) &= (q^3 - q^2 + (q^3 - q^2) \chi^{-1}(\varpi)) f_1 + (q^3 - q^2) f_2 + q \chi(\varpi) f_4, \\ L'_I(f_4) &= (q^4 - q^3) \chi^{-1}(\varpi) f_1 + q^3 f_3. \end{aligned}$$

Hence the eigenvalues of  $L'_I$  on  $V_\rho$  are  $\pm q^2 \sigma(\varpi), \pm q^2 \chi \sigma(\varpi)$ .

2.3.2. *Type IIIa.* Suppose  $\rho \simeq \chi \rtimes \sigma \mathrm{St}_{\mathrm{GSp}_2}$ , which is the unique quotient of the representation  $\chi \times \nu^{-1} \rtimes \nu^{\frac{1}{2}}\sigma$ . Following the same argument as in type IIa and applying results from §1.0.1 with  $\chi_1 = \chi$  and  $\chi_2 = \nu^{-1}$ , we deduce that the eigenvalues of  $L'_I$  on  $V_\rho^I$  are  $\pm q \sigma(\varpi), \pm q \chi \sigma(\varpi)$ .

2.4. **Type IV representations.** Suppose  $\rho$  is of type IV, then it is a constituent of  $\nu^{-2} \times \nu^{-1} \rtimes \nu^{\frac{3}{2}}\sigma$ . There are four constituents in  $\nu^{-2} \times \nu^{-1} \rtimes \nu^{\frac{3}{2}}\sigma$  corresponding to representations of types IVa- IVd. We shall not concern representations of types IVb and IVc as they will never occur in  $L^2(\Gamma \backslash G/Z)$ .

2.4.1. *Type IVd.* In this case  $\rho \simeq \sigma \mathbf{1}_{\mathrm{GSp}_4}$  with  $\sigma^2 = \mathbf{1}_{F^\times}$ , which is a one-dimensional representation, and can be regarded as a subrepresentation of  $\nu^{-2} \times \nu^{-1} \rtimes \nu^{\frac{3}{2}}\sigma$ . Following the notation in §1 and using the results there with  $\chi_1, \chi_2, \sigma$  in the inducing data equal to  $\nu^{-2}, \nu^{-1}$  and  $\nu^{\frac{3}{2}}\sigma$  respectively, it is easy to observe that  $V_\rho^I$  is generated by the single function  $\sum_{i=1}^8 f_i$ , and the eigenvalues of  $L'_I$  restricted on  $V_\rho$  is  $q^3$ .

2.4.2. *Type IVa.* Suppose  $\rho \simeq \sigma \mathrm{St}_{\mathrm{GSp}_4}$  with  $\sigma^2 = \mathbf{1}_{F^\times}$ . It can be regarded as a subrepresentation of  $\nu^2 \times \nu \rtimes \nu^{-\frac{3}{2}}\sigma$ . As in §1, we realize the principal series representation  $\nu^2 \times \nu \rtimes \nu^{-\frac{3}{2}}\sigma$  in the standard model  $V$  and use the same notation  $f_\alpha$  for the function in  $V$  supported on  $B\alpha I$  with  $f(\alpha I) = 1$ . The space  $V_\rho^I$  has dimension one generated by  $q^4 f_1 - q^3 f_2 - q^3 f_3 + q^2 f_4 + q^2 f_5 - q f_6 - q f_7 + f_8$ . Direct computation shows that the eigenvalue of  $L'_I$  on  $V_\rho^I$  is  $-1$ .

2.5. **Type V representations.** Representations of type V are the constituents of  $\nu \xi \times \xi \rtimes \nu^{-1/2}\sigma$ . There are four constituents in  $\nu \xi \times \xi \rtimes \nu^{-1/2}\sigma$  corresponding to types Va -Vd.

2.5.1. *Types Vb and Vc.* We consider types Vb and Vc together since  $L(\nu^{1/2} \xi \mathrm{St}_{\mathrm{GL}_2}, \nu^{-1/2}\sigma)$  and  $L(\nu^{1/2} \xi \mathrm{St}_{\mathrm{GL}_2}, \xi \nu^{-1/2}\sigma)$  are twists of each other. Suppose  $\rho \simeq L(\nu^{1/2} \xi \mathrm{St}_{\mathrm{GL}_2}, \nu^{-1/2}\sigma)$  with  $\sigma^2 = \mathbf{1}_{F^\times}$ , then  $\rho$  can be regarded as a subrepresentation in  $\nu^{\frac{1}{2}} \xi \mathbf{1}_{\mathrm{GL}_2} \rtimes \nu^{-\frac{1}{2}} \xi \sigma$ . Since  $\nu^{\frac{1}{2}} \xi \mathbf{1}_{\mathrm{GL}_2} \rtimes \nu^{-\frac{1}{2}} \xi \sigma$  is parabolically induced from a character on  $P$ , we realize it in the standard induced model  $V$  as usual, and identify  $V_\rho$  as a subspace in  $V$ . A basis for  $V_\rho^I$  has been given explicitly in Schmidt [3, Corollary 2.6 (ii)] and recorded also in [1]. Let  $f_\alpha(x)$  be the function in  $V$  supported on  $P\alpha I$  with  $f_\alpha(\alpha I) = 1$ . Then the functions  $f_1 := f_{id}, f_2 := f_{s_2}, f_3 := f_{s_2s_1}$ , and  $f_4 := f_{s_2s_1s_2}$  form a basis of

$V^I$  just as in the case of type IIb. Then The space  $V_\rho^I$  is generated by  $\phi_1 = q^2 f_1 + q^2 f_2 - f_3 - f_4$  and  $\phi_2 = (q^3 + q^2)f_1 + (q^2 - q)f_2 + (q^2 - q)f_3 - (q + 1)f_4$ .

In terms of this chosen basis, the action of  $L'_I$  is given by  $L'_I(\phi_1) = q^2 \phi_1 - q \phi_2$ ,  $L'_I(\phi_2) = -q \phi_2$ . Hence the eigenvalues of  $L'_I$  on  $V_\rho^I$  are  $-q, q^2$ , and the result is the same for  $\rho' \simeq L(\nu^{1/2} \xi \text{St}_{\text{GL}_2}, \xi \nu^{-1/2} \sigma) \simeq \xi \rho$ .

**2.5.2. Type Vd.** Consider  $\rho \simeq L(\nu \xi, \xi \rtimes \nu^{-1/2} \sigma)$  with  $\sigma^2 = \mathbf{1}_{F^\times}$ , then  $\rho$  can be regarded as a subrepresentation in  $\nu^{-\frac{1}{2}} \xi \mathbf{1}_{\text{GL}_2} \rtimes \nu^{\frac{1}{2}} \xi \sigma$ . Similar to §2.5.1, we realize  $\nu^{-\frac{1}{2}} \xi \mathbf{1}_{\text{GL}_2} \rtimes \nu^{\frac{1}{2}} \xi \sigma$  in the standard induced model  $V$  and identify  $V_\rho$  as a subspace in  $V$ . Define a basis  $f_1, \dots, f_4$  of  $V^I$  similarly. It follows from [3, Proposition 2.5 (ii)] that  $V_\rho^I$  is generated by  $\phi_1 = \frac{1}{2}(q^2 + 1)f_1 - \frac{1}{2}(q - 1)f_2 - \frac{1}{2}(q - 1)f_3 + f_4$  and  $\phi_2 = -\frac{1}{2}(q^2 - q)f_1 + qf_2 + qf_3 + \frac{1}{2}(q - 1)f_4$ . Explicit calculation then shows that the eigenvalues of  $L'_I$  on  $V_\rho^I$  are  $-q^2, -q^2$ .

**2.5.3. Type Va.** Suppose  $\rho \simeq \delta([\xi, \nu \xi], \nu^{-1/2} \sigma)$  with  $\sigma^2 = \mathbf{1}_{F^\times}$ . As this is the only remaining case in Group V, the eigenvalues for  $L'I$  on  $V_\rho$  can be determined by applying result from §1.0.1, §2.5.1, §2.5.2 with the inducing data  $\chi_1, \chi_2, \sigma$  being  $\nu \xi, \xi$ , and  $\nu^{-\frac{1}{2}} \sigma$  respectively. Then we see that the eigenvalues of  $L'_I$  on  $V_\rho^I$  are  $q, q$ .

**2.6. Type VI representations.** Representations in type VI are constituents of  $\nu \times \mathbf{1}_{F^\times} \rtimes \nu^{-\frac{1}{2}} \sigma$ . When  $\rho$  is of type VIb, VIc, or VId, a basis for  $V_\rho^I$  has been obtained in Schmidt [3] by studying appropriate intertwining operators, which makes explicit calculation possible. Once the eigenvalues from types VIb, VIc, VId are known, we then apply results in §1.0.1 to determine the eigenvalues from the remaining type VIa case, just like the work done before.

**2.6.1. Type VIb.** Consider  $\rho \simeq \tau(T, \nu^{-1/2} \sigma)$  with  $\sigma^2 = \mathbf{1}_{F^\times}$ . Then  $\rho$  can be regarded as a subrepresentation in  $\nu^{\frac{1}{2}} \mathbf{1}_{\text{GL}_2} \rtimes \nu^{-\frac{1}{2}} \sigma$ . We realize  $\nu^{\frac{1}{2}} \mathbf{1}_{\text{GL}_2} \rtimes \nu^{-\frac{1}{2}} \sigma$  in the standard induced model  $V$  and identify  $V_\rho$  as a subspace in  $V$ . Let  $f_1, \dots, f_4$  be the functions in  $V^I$  defined as in the case of type IIb. According to [3, Corollary 2.6], the space  $V_\rho^I$  is 1-dimensional, generated by the function  $q^2 f_1 - q f_2 - q f_3 + f_4$ . The eigenvalue of  $L'_I$  on  $V_\rho^I$  is  $q$ .

**2.6.2. Type VIc.** Suppose  $\rho \simeq L(\nu^{\frac{1}{2}} \text{St}_{\text{GL}_2}, \nu^{-\frac{1}{2}} \sigma)$  with  $\sigma^2 = \mathbf{1}_{F^\times}$ . Then  $\rho$  can be regarded as a subrepresentation of  $\mathbf{1}_{F^\times} \rtimes \sigma \mathbf{1}_{\text{GL}_2}$ . Realize  $\mathbf{1}_{F^\times} \rtimes \sigma \mathbf{1}_{\text{GL}_2}$  in the standard induced model  $V$  and let  $f_1, \dots, f_4$  be the functions in  $V^I$  defined as in the case of type IIIb. By [3, Corollary 3.6],  $V_\rho^I$  is generated by the function  $q^2 f_1 - q f_2 - q f_3 + f_4$ . The eigenvalue of  $L'_I$  on  $V_\rho^I$  is  $q\sigma(\varpi)$ .

**2.6.3. Type VId.** Suppose  $\rho \simeq L(\nu, \mathbf{1}_{F^\times} \rtimes \nu^{-\frac{1}{2}} \sigma)$  with  $\sigma^2 = \mathbf{1}_{F^\times}$ . Then  $\rho$  is a subrepresentation of  $\nu^{-\frac{1}{2}} \mathbf{1}_{\text{GL}_2} \rtimes \nu^{\frac{1}{2}} \sigma$ , which again is realized in the standard induced model  $V$ . Let  $f_1, \dots, f_4$  be the functions in  $V_I$  defined as in the case of type IIb. Examining the kernel of the intertwining operator in [3, Proposition 2.5] shows that the space  $V_\rho^I$  has as a basis  $f_1 + f_2, f_3 + f_4$  and  $q f_1 + f_3$ . The eigenvalues of  $L'_I$  on  $V_\rho^I$  are  $-q^2, q^2, q^2$ .

**2.6.4. Type VIa.** Suppose  $\rho \simeq \tau(S, \nu^{-\frac{1}{2}} \sigma)$  with  $\sigma^2 = \mathbf{1}_{F^\times}$ . The eigenvalues of  $L'_I$  on  $V_\rho^I$  are  $q, -q, -q$ .

### 3. SUMMARY

We summarize the computations above in the following table. For each type of representation  $(\rho, V_\rho)$ , the column  $-L'_I$  shows the eigenvalues of  $-L'_I$ , which are the reciprocals of the zeros of  $\det(I + L'_I u)$  arising from  $\rho$ . Similarly, the column  $\pm L_{P_1}$  shows the reciprocals of the zeros of  $\det(I - L_{P_1}^2 u^2)$ , the column  $L_{P_2}$  shows the reciprocals of the zeros of  $\det(I - L_{P_1} u)$ , and the column

$A_1, A'_2, A''_2$  records the reciprocals of the zeros of  $\det(I - A'_2 u + (qA_1^2 - 2q^2 A''_2)u^2 - q^4 A'_2 u^3 + q^8 I u^4)$  arising from  $\rho$ . The column  $R(u)$  records the contribution of each representation  $\rho$  to  $R(u)$ .

| type | $-L'_I$                                                                                                                                                                                  | $\pm L_{P_1}$                                                                                                                                                                            | $L_{P_2}$                                                                                                                                        | $A_1, A'_2, A''_2$                                                                                                                               | condition                             | $R(u)$            |
|------|------------------------------------------------------------------------------------------------------------------------------------------------------------------------------------------|------------------------------------------------------------------------------------------------------------------------------------------------------------------------------------------|--------------------------------------------------------------------------------------------------------------------------------------------------|--------------------------------------------------------------------------------------------------------------------------------------------------|---------------------------------------|-------------------|
| I    | $\pm q^{\frac{3}{2}} \chi_1 \sigma(\varpi)$<br>$\pm q^{\frac{3}{2}} \chi_2 \sigma(\varpi)$<br>$\pm q^{\frac{3}{2}} \chi_1 \chi_2 \sigma(\varpi)$<br>$\pm q^{\frac{3}{2}} \sigma(\varpi)$ | $\pm q^{\frac{3}{2}} \chi_1 \sigma(\varpi)$<br>$\pm q^{\frac{3}{2}} \chi_2 \sigma(\varpi)$<br>$\pm q^{\frac{3}{2}} \chi_1 \chi_2 \sigma(\varpi)$<br>$\pm q^{\frac{3}{2}} \sigma(\varpi)$ | $q^2 \chi_1 \sigma^2(\varpi)$<br>$q^2 \chi_2 \sigma^2(\varpi)$<br>$q^2 \chi_1 \chi_2 \sigma^2(\varpi)$<br>$q^2 \chi_1^2 \chi_2 \sigma^2(\varpi)$ | $q^2 \chi_1 \sigma^2(\varpi)$<br>$q^2 \chi_2 \sigma^2(\varpi)$<br>$q^2 \chi_1 \chi_2 \sigma^2(\varpi)$<br>$q^2 \chi_1^2 \chi_2 \sigma^2(\varpi)$ | $\chi_1 \chi_2 \sigma^2 = \mathbf{1}$ | 1                 |
| IIa  | $\pm q$<br>$q^{\frac{3}{2}} \chi(\varpi), q^{\frac{3}{2}} \chi^{-1}(\varpi)$                                                                                                             | $\pm q$                                                                                                                                                                                  | $q^{\frac{3}{2}} \chi^{-1}(\varpi)$<br>$q^{\frac{3}{2}} \chi(\varpi)$                                                                            | none                                                                                                                                             | $\chi^2 \sigma^2 = \mathbf{1}$        | 1                 |
| IIb  | $\pm q^2$<br>$-q^{\frac{3}{2}} \chi(\varpi), -q^{\frac{3}{2}} \chi^{-1}(\varpi)$                                                                                                         | $\pm q^{\frac{3}{2}} \chi^2 \sigma(\varpi)$<br>$\pm q^{\frac{3}{2}} \sigma(\varpi)$<br>$\pm q^2$                                                                                         | $q^{\frac{5}{2}} \chi(\varpi)$<br>$q^{\frac{5}{2}} \chi^{-1}(\varpi)$<br>$q^2 \chi^{-1}(\varpi)$                                                 | $q^{\frac{5}{2}} \chi(\varpi)$<br>$q^{\frac{5}{2}} \chi^{-1}(\varpi)$<br>$q^{\frac{3}{2}} \chi(\varpi), q^{\frac{3}{2}} \chi^{-1}(\varpi)$       | $\chi^2 \sigma^2 = \mathbf{1}$        | 1                 |
| IIIa | $\pm q \chi \sigma(\varpi)$<br>$\pm q \sigma(\varpi)$                                                                                                                                    | $\pm q \chi \sigma(\varpi)$<br>$\pm q \sigma(\varpi)$                                                                                                                                    | $q$                                                                                                                                              | none                                                                                                                                             | $\chi \sigma^2 = \mathbf{1}$          | $(1 - qu)^{-1}$   |
| IIIb | $\pm q^2 \chi \sigma(\varpi)$<br>$\pm q^2 \sigma(\varpi)$                                                                                                                                | $\pm q^2 \chi \sigma(\varpi)$<br>$\pm q^2 \sigma(\varpi)$                                                                                                                                | $q^3$<br>$q^2 \chi(\varpi), q^2 \chi^{-1}(\varpi)$                                                                                               | $q, q^3$<br>$q^2 \chi(\varpi), q^2 \chi^{-1}(\varpi)$                                                                                            | $\chi \sigma^2 = \mathbf{1}$          | $1 - qu$          |
| IVa  | 1                                                                                                                                                                                        | none                                                                                                                                                                                     | none                                                                                                                                             | none                                                                                                                                             | $\sigma^2 = \mathbf{1}$               | $1 - u$           |
| IVd  | $-q^3$                                                                                                                                                                                   | $\pm q^3$                                                                                                                                                                                | $q^4$                                                                                                                                            | $q^4, q^3, q, 1$                                                                                                                                 | $\sigma^2 = \mathbf{1}$               | $(1 - qu)(1 - u)$ |
| Va   | $-q, -q$                                                                                                                                                                                 | none                                                                                                                                                                                     | $-q$                                                                                                                                             | none                                                                                                                                             | $\sigma^2 = \mathbf{1}$               | $1 + qu$          |
| Vb   | $-q^2, q$                                                                                                                                                                                | $\pm q$                                                                                                                                                                                  | $-q^2$                                                                                                                                           | none                                                                                                                                             | $\sigma^2 = \mathbf{1}$               | $(1 + qu)^{-1}$   |
| Vc   | $-q^2, q$                                                                                                                                                                                | $\pm q$                                                                                                                                                                                  | $-q^2$                                                                                                                                           | none                                                                                                                                             | $\sigma^2 = \mathbf{1}$               | $(1 + qu)^{-1}$   |
| Vd   | $q^2, q^2$                                                                                                                                                                               | $\pm q^2, \pm q^2$                                                                                                                                                                       | $-q^3$                                                                                                                                           | $-q^3, -q^2, -q^2, -q$                                                                                                                           | $\sigma^2 = \mathbf{1}$               | $1 + qu$          |
| VIa  | $\pm q, q$                                                                                                                                                                               | $\pm q$                                                                                                                                                                                  | $q$                                                                                                                                              | none                                                                                                                                             | $\sigma^2 = \mathbf{1}$               | 1                 |
| VIb  | $-q$                                                                                                                                                                                     | $\pm q$                                                                                                                                                                                  | none                                                                                                                                             | none                                                                                                                                             | $\sigma^2 = \mathbf{1}$               | $(1 - qu)^{-1}$   |
| VIc  | $q^2$                                                                                                                                                                                    | none                                                                                                                                                                                     | $q^2$                                                                                                                                            | none                                                                                                                                             | $\sigma^2 = \mathbf{1}$               | 1                 |
| VIId | $q^2, -q^2, -q^2$                                                                                                                                                                        | $\pm q^2, \pm q^2$                                                                                                                                                                       | $q^3, q^2$                                                                                                                                       | $q^3, q^2, q^2, q$                                                                                                                               | $\sigma^2 = \mathbf{1}$               | $1 - qu$          |

## REFERENCES

- [1] Y. Fang, W.-C. W. Li, and C.-J. Wang, *The zeta functions of complexes from  $\mathrm{Sp}(4)$* , Int. Math. Res. Not. **4** (2013), 886–923.
- [2] M.-H. Kang, W.-C. W. Li, and C.-J. Wang, *Zeta and L-functions of finite quotients of apartments and buildings*, submitted (2016).
- [3] R. Schmidt, *On classical Saito-Kurokawa liftings*, J. Reine Angew Math. **604** (2007), 211–236.
